# Supplementary material for: Convergence and Diversity in the Control Hierarchy
Source: arXiv:2306.03628 source file (2023-06-06)
Supplement: Supplementary file 1 [file appendix.tex]

\subsection{PDA $\control$ CFG}

\begin{defin}
Let $\grammar = (\nonterm, \alphabet, \labelset, \rules, \ntvar{S})$ be a weighted LD-CFG over the monoid $\wtkleene{\alphabet}$ and $\pushdown = (\states, \labelset, \stackalphabet, \trans, (q_\init, \NTvar{S}),(q_\final, \varepsilon))$ a controller PDA, both in normal form. $\grammar$ controlled by $\pushdown$ is a formal system $(\carrierset,\yield)$, where $\carrierset = \nonterm[\states \times \kleene{\stackalphabet}] \times \wtkleene{\alphabet}$ and the yield function $\yield \colon \carrierset \rightharpoonup \wtkleene{\alphabet}$ is defined as $\yield((\ntvar{X}[p,\stackseq],\str)) = \str$ if $\ntvar{X}=\ntvar{S}, p=q_\init,\stackseq=\NTvar{S}$. 

The signature $\signature$ is constructed as follows:
\begin{itemize}
    \item For each production $\ntvar{X}[p, \NTvar{A}]\outarrow \symvar{a}$, which we label with $\pi$, add a nullary operation $\pi()=(\ntvar{X}[p,\NTvar{A}],\symvar{a})$;
    \item For each production $\ntvar{X}[p, \rest \NTvar{A}]\rightarrow \ntvar{X}[q, \rest \stackseq'], |\stackseq'|\leq 2$, which we label with $\pi$, add a unary operation $\pi((\ntvar{X}[q,\stackseq \stackseq'],\str))=(\ntvar{X}[p,\stackseq \NTvar{A}],\str)$;
    \item For each production $\ntvar{X}[p, \rest \NTvar{A}]\outarrow \ntvar{Y}[q, \rest]$, which we label with $\pi$, add a unary operation $\pi((\ntvar{Y}[q,\stackseq],\str))=(\ntvar{X}[p,\stackseq \NTvar{A}],\str)$;
    \item For each production $\ntvar{X}[p, \rest \NTvar{A}]\outarrow \ntvar{Y}[q, \rest] \ntvar{Z}[q_\init, \NTvar{S}]$, which we label with $\pi$, add a binary operation $\pi((\ntvar{Y}[q,\stackseq],\str), (\ntvar{Z}[q_\init,\NTvar{S}],\str))=(\ntvar{X}[p,\stackseq \NTvar{A}],\str)$;
    \item For each production $\ntvar{X}[p, \rest \NTvar{A}]\outarrow \ntvar{Y}[q_\init, \NTvar{S}] \ntvar{Z}[q, \rest]$, which we label with $\pi$, add a binary operation $\pi((\ntvar{Y}[q_\init,\NTvar{S}],\str),(\ntvar{Z}[q,\stackseq],\str))=(\ntvar{X}[p,\stackseq \NTvar{A}],\str)$;
\end{itemize}

\end{defin}

\subsection{PDA $\control$ PDA}

\begin{defin}
Let $\pushdown_1 = (\states, \alphabet, \labelset, \stackalphabet, \trans, (q_\init, \ntvar{S}),(q_\final, \varepsilon))$ be a weighted LD-PDA in normal form over the monoid $\wtkleene{\alphabet}$ and $\pushdown_2 = (\states', \labelset, \stackalphabet', \trans', (q'_\init, \NTvar{S}),(q'_\final, \varepsilon))$ a controller PDA in normal form. $\pushdown_1$ controlled by $\pushdown_2$ is a formal system $(\carrierset,\yield)$, where $\carrierset = \states \times \kleene{(\stackalphabet [\states' \times \kleene{\stackalphabet'}])}\times \wtkleene{\alphabet}$ and the yield function $\yield \colon \carrierset \rightharpoonup \wtkleene{\alphabet}$ is defined as $\yield (p, \nestedstack, \str) = \str$ if $p=q_\init, \nestedstack = \ntvar{S}[q'_\init,\NTvar{S}]$. The signature $\signature$ is constructed as follows:
\begin{itemize}
    \item $\signature$ contains a nullary operation $\init()=(q_\final, \varepsilon,\varepsilon)$;
    \item For each transition $\atrans = p, \nestedstack \ntvar{X}[r, \rest \NTvar{A}] \xrightarrow{\str} p, \nestedstack \ntvar{X}[t, \rest \stackseq], |\stackseq|\leq 2$ add a unary operation $\atrans (p,\nestedstack \ntvar{X}[t, \stackseq' \stackseq],\str) = (p, \nestedstack \ntvar{X}[r, \stackseq' \NTvar{A}],\str)$;
    \item For each transition $\atrans = p, \nestedstack \ntvar{X}[r, \rest \NTvar{A}] \xoutarrow{\str} q, \nestedstack \ntvar{Y}[t, \rest]$ add a unary operation $\atrans(q,\nestedstack \ntvar{Y}[t, \stackseq],\str) = (p, \nestedstack \ntvar{X}[r, \stackseq \NTvar{A}],\str)$;
    \item For each transition $\atrans = p, \nestedstack \ntvar{X}[r, \rest \NTvar{A}] \xoutarrow{\str} q, \nestedstack \ntvar{Y}[t, \rest ] \ntvar{Z}[q'_\init,\NTvar{S}]$ add a unary operation 
    $\atrans(q,\nestedstack \ntvar{Y}[t, \stackseq] \ntvar{Z}[q'_\init,\NTvar{S}],\str) =(p, \nestedstack \ntvar{X}[r, \stackseq \NTvar{A}],\str)$;
    \item For each transition $\atrans = p, \nestedstack \ntvar{X}[r, \rest \NTvar{A}] \xoutarrow{\str} q, \nestedstack \ntvar{Y}[q'_\init,\NTvar{S}] \ntvar{Z}[t, \rest]$ add a unary operation 
    $\atrans(q,\nestedstack \ntvar{Y}[q'_\init,\NTvar{S}] \ntvar{Z}[t, \stackseq],\str) = 
    (p, \nestedstack \ntvar{X}[r, \stackseq \NTvar{A}],\str)$;
    \item For each transition $\atrans = p, \nestedstack \ntvar{X}[r, \NTvar{A}] \xoutarrow{\str} q, \nestedstack$ add a unary operation 
    $\atrans^{\pushdown} (q,\nestedstack,\str)= (p, \nestedstack \ntvar{X}[r,\NTvar{A}],\str)$;
\end{itemize}
Let $\pushdown_1 = (\states_1, \alphabet, \labelset, \stackalphabet_1, \trans_1, (q_{0,1}, \ntvar{S}),(q_{f,1}, \varepsilon))$ be an LD-PDA and $\pushdown_2 = (\states_2, \labelset, \stackalphabet_2, \trans_2, (q_{0,2}, \NTvar{S}),(q_{f,2}, \varepsilon))$ be a controller PDA. $\pushdown_1$ controlled by $\pushdown_2$ is a formal system $\pushdown$ with carrier set $\carrierset = \states_1 \times \stackalphabet_1[\stackalphabet_1 \cup \{\varepsilon \}] \times \states_1 \times \states_2 \times \stackalphabet_2 \times \states_2 \times \kleene{\alphabet}$. The yield function $\yield$ maps $(q_{0,1},\ntvar{S}[\varepsilon],q_{f,1},q_{0,2},\NTvar{S},q_{f,2},w)$ to $w$.
\end{defin}

\subsection{CFG $\control$ PDA}

Let $\pushdown=(\states,\alphabet,\labelset,\stackalphabet,\trans,(q_\init,\ntvar{S}),(q_\final,\varepsilon))$ be a weighted LD-PDA in normal form over the monoid $\wtkleene{\alphabet}$ and $\grammar=(\nonterm,\labelset,\rules,\NTvar{S})$ a controller CFG in normal form. $\pushdown$ controlled by $\grammar$ is a formal system $(\carrierset,\yield)$ where $\carrierset=\states\times \kleene{(\stackalphabet[\kleene{(\nonterm \cup \labelset)}])}\times \wtkleene{\alphabet})$ and the yield function $\yield$ is defined as $\yield (p,\ntvar{X}[\sent],\str)=\str$ if $p=q_\init$, $\ntvar{X}=\ntvar{S}$ and $\sent=\NTvar{S}$. The signature $\signature$ is constructed as follows: 
\begin{itemize}
    \item $\signature$ contains a nullary operation $\init()=(q_\final,\varepsilon,\varepsilon)$;
    \item For each transition $\atrans=(p,\nestedstack \ntvar{X}[\ell]\xoutarrow{\symvar{a}}q,\nestedstack)$, $\signature$ contains a unary operation $\atrans((q,\nestedstack,\str))=(p,\nestedstack\ntvar{X}[\ell],\symvar{a}\str)$;
    \item For each transition $\atrans=(p,\nestedstack \ntvar{X}[\ell\rest]\xoutarrow{\varepsilon}q,\nestedstack\ntvar{Y}[\rest])$, $\signature$ contains a unary operation $\atrans((q,\nestedstack\ntvar{Y}[\sent],\str))=(p,\nestedstack\ntvar{X}[\ell\sent],\str)$;
    \item For each transition $\atrans=(p,\nestedstack \ntvar{X}[\ell\rest]\xoutarrow{\varepsilon}q,\nestedstack\ntvar{Y}[\rest]\ntvar{Z}[\NTvar{S}])$, $\signature$ contains a unary operation $\atrans((q,\nestedstack\ntvar{Y}[\sent]\ntvar{Z}[\NTvar{S}],\str))=(p,\nestedstack\ntvar{X}[\ell\sent],\str)$;
    \item For each transition $\atrans=(p,\nestedstack \ntvar{X}[\ell\rest]\xoutarrow{\varepsilon}q,\nestedstack\ntvar{Y}[\NTvar{S}]\ntvar{Z}[\rest])$, $\signature$ contains a unary operation $\atrans((q,\nestedstack\ntvar{Y}[\NTvar{S}]\ntvar{Z}[\sent],\str))=(p,\nestedstack\ntvar{X}[\ell\sent],\str)$;
    \item For each transition $\atrans=(p,\nestedstack \ntvar{X}[\NTvar{A}\rest]\xoutarrow{\varepsilon}q,\nestedstack\ntvar{X}[\ell\rest])$, $\signature$ contains a unary operation $\atrans((q,\nestedstack\ntvar{X}[\ell\sent],\str))=(p,\nestedstack\ntvar{X}[\NTvar{A}\sent],\str)$;
    \item For each transition $\atrans=(p,\nestedstack \ntvar{X}[\NTvar{A}\rest]\xoutarrow{\varepsilon}q,\nestedstack\ntvar{X}[\sent'\rest]),\sent'\in\kleene{\nonterm},|\sent'|\leq 2$, $\signature$ contains a unary operation $\atrans((q,\nestedstack\ntvar{X}[\sent'\sent],\str))=(p,\nestedstack\ntvar{X}[\NTvar{A}\sent],\str)$;
\end{itemize}

\section{\BijeqNN{}}\label{app:d-weak-eq}

We prove that the four formalisms obtained by mixing an LD-CFG or LD-PDA with either a CFG or PDA are \bijeqJJ{}.

\begin{proposition} \label{prop:ldcfg-cfg-eq-ldcfg-pda}
An LD-CFG controlled by a CFG is \bijeqJJ{} to an LD-CFG controlled by a PDA.
\end{proposition}

\begin{proof}
$(\Rightarrow)$ Let $\grammar$ be an LD-CFG, $\grammar'=(\nonterm,\alphabet,\rules,\NTvar{S})$ a controller CFG and $\yield$ the yield of $\grammar$ controlled by $\grammar'$. We can construct a controller PDA $\pushdown=(\{p\},\alphabet,\nonterm,\trans,(p,\NTvar{S}),(p,\varepsilon))$, with yield $\yield'$, such that $\grammar$ controlled by $\pushdown$ is \bijeqJJ{} to $\grammar$ controlled by $\grammar'$. For a controller CFG in normal form with productions 
\begin{align*}
    \NTvar{A} &\rightarrow \NTvar{BC},\\
    \NTvar{A} &\rightarrow \NTvar{B},\\
    \NTvar{A} &\rightarrow \ell,\\
    \NTvar{A} &\rightarrow \varepsilon,
\end{align*}
the set $\trans$ contains the transitions
\begin{align*}
    p,\NTvar{A} &\xrightarrow{\varepsilon}p, \NTvar{BC},\\
    p,\NTvar{A} &\xrightarrow{\varepsilon}p, \NTvar{B},\\
    p,\NTvar{A} &\xrightarrow{\ell}p, \varepsilon,\\
    p,\NTvar{A} &\xrightarrow{\varepsilon}p,\varepsilon.
\end{align*}
The function $\phi\colon \dom{}(\yield)\rightarrow\dom{}(\yield')$ is defined as $\phi((\ntvar{S}[\NTvar{S}],\str))=(\ntvar{S}[p,\NTvar{S}],\str)$.

We need to prove that for every derivation of the string $\str$ in $\grammar$ controlled by $\grammar'$, there is a derivation of $\str$ in $\grammar$ controlled by $\pushdown$. Since the LD-CFG $\grammar$ is the same in both formal systems, the same productions of $\grammar$ will be applied whenever $\grammar'$ produces a label $\ell$ and $\pushdown$ scans an $\ell$. It suffices to show that the labels are produced/scanned by both in the same order. This is true since $\grammar'$ and $\pushdown$ have the same language.
\alexandra{this could be made more formal but then we would need to define what a derivation is in each of these algebras}

$(\Leftarrow)$ Let $\grammar$ be an LD-CFG, $\pushdown=(\states,\alphabet,\stackalphabet,\trans,(q_\init,\NTvar{S}),(q_\final,\varepsilon))$ a controller PDA and $\yield$ the yield of $\grammar$ controlled by $\pushdown$. We can construct a controller CFG $\grammar'=(\nonterm,\alphabet,\rules,\NTvar{S})$, with yield $\yield'$, such that $\grammar$ controlled by $\grammar'$ is \bijeqJJ{} to $\grammar$ controlled by $\pushdown$. The nonterminal set is defined as $\nonterm =\{\NTvar{A}_{pq} \mid \NTvar{A}\in \stackalphabet, p,q \in \states \}$ and $\trans$ contains transitions of the form
\begin{align*}
    \NTvar{A}_{pt} &\rightarrow \NTvar{B}_{qr} \NTvar{C}_{rt},\quad \forall r,t \in \states\\
    \NTvar{A}_{pr} &\rightarrow \NTvar{B}_{qr},\quad \forall r \in \states \\
    \NTvar{A}_{pq} &\rightarrow \Symvar{a}\\
    \NTvar{A}_{pq} &\rightarrow \varepsilon.
\end{align*}
The function $\phi\colon \dom{}(\yield)\rightarrow\dom{}(\yield')$ is defined as $\phi((\ntvar{S}[q_\init,\NTvar{S}],\str))=(\ntvar{S}[\NTvar{S}_{q_\init q_\final}],\str)$.
Similar to the previous direction of the proof, $\grammar'$ and $\pushdown$ generate/recognize the same language, therefore the rules of $\grammar$ will be applied in the same order, generating the same strings $\str$.
\end{proof}

\begin{proposition} \label{prop:ldcfg-pda-eq-ldpda-pda}
An LD-CFG controlled by a PDA is \bijeqJJ{} to an LD-PDA controlled by a PDA.
\end{proposition}

\begin{proof}

$(\Rightarrow)$ 
Let $\grammar=(\nonterm,\alphabet,\labelset,\rules,\ntvar{S})$ be an LD-CFG, $\pushdown$ a controller PDA and $\yield$ the yield of $\grammar$ controlled by $\pushdown$. We can construct an LD-PDA $\pushdown'$ controlled by $\pushdown$, with yield $\yield'$, that is \bijeqJJ{} to $\grammar$ controlled by $\pushdown$. We define $\pushdown=( \{ p \},\alphabet,\nonterm,\labelset,\trans,(p,\ntvar{S}),(p,\varepsilon))$. For an LD-CFG in normal form with productions $\rules$
\begin{align*}
    \ell_1 \colon \ntvar{X} &\rightarrow \dist{\ntvar{Y}} \ntvar{Z},\\
    \ell_2 \colon \ntvar{X} &\rightarrow \ntvar{Y} \dist{\ntvar{Z}},\\
    \ell_3 \colon \ntvar{X} &\rightarrow \dist{\ntvar{Y}},\\
    \ell_4 \colon \ntvar{X} &\rightarrow \symvar{a},\\
    \ell_5 \colon \ntvar{X} &\rightarrow \varepsilon,
\end{align*}
we define the set of transitions $\trans$ as
\begin{align*}
    \ell_1 \colon p,\ntvar{X} &\xrightarrow{\varepsilon} p,\dist{\ntvar{Y}} \ntvar{Z},\\
    \ell_2 \colon p,\ntvar{X} &\xrightarrow{\varepsilon} p,\ntvar{Y} \dist{\ntvar{Z}},\\
    \ell_3 \colon p,\ntvar{X} &\xrightarrow{\varepsilon} p,\dist{\ntvar{Y}},\\
    \ell_4 \colon p,\ntvar{X} &\xrightarrow{\symvar{a}} p,\varepsilon,\\
    \ell_5 \colon p,\ntvar{X} &\xrightarrow{\varepsilon} p,\varepsilon.
\end{align*}
We define the function $\phi \colon \dom{}(\yield) \rightarrow \dom{}(\yield')$ as $\phi (\ntvar{S}[q_\init,\NTvar{S}],\str)=(p,\ntvar{S}[q_\init,\NTvar{S}],\str)$.

$(\Leftarrow)$ 
Let $\pushdown=(\states,\alphabet,\nonterm,\labelset,\trans,(q_\init,\ntvar{S}), (q_\final,\varepsilon))$ be an LD-PDA, $\pushdown'$ a controller PDA and $\yield$ the yield of $\pushdown$ controlled by $\pushdown'$. We can construct an LD-CFG $\grammar$ controlled by $\pushdown'$, with yield $\yield'$, that is \bijeqJJ{} to $\pushdown$ controlled by $\pushdown'$. We define $\grammar=(\nonterm,\alphabet,\labelset,\rules,\ntvar{S})$, where $\nonterm = \{\ntvar{X}_{pq} \mid \ntvar{X} \in \stackalphabet, p,q \in \states \}$. The set of productions $\rules$ of $\grammar$ can be constructed as follows:
\begin{itemize}
    \item For each transition $\ell \colon p,\ntvar{X} \xrightarrow{\symvar{a}} q,\varepsilon$ add a production $\ell \colon \ntvar{X}_{pq} \rightarrow \symvar{a}$;
    \item For each transition $\ell \colon p,\ntvar{X} \xrightarrow{\varepsilon} q, \dist{\ntvar{Y}}$ add productions $\ell \colon \ntvar{X}_{pr} \rightarrow \dist{\ntvar{Y}}_{qr},\forall r \in \states$;
    \item For each transition $\ell \colon p,\ntvar{X} \xrightarrow{\varepsilon} q, \dist{\ntvar{Y}} \ntvar{Z}$ add productions $\ell \colon \ntvar{X}_{pt} \rightarrow \dist{\ntvar{Y}}_{qr} \ntvar{Z}_{rt},\forall r,t \in \states$;
    \item For each transition $\ell \colon p,\ntvar{X} \xrightarrow{\varepsilon} q, \ntvar{Y} \dist{\ntvar{Z}}$ add productions $\ell \colon \ntvar{X}_{pt} \rightarrow \ntvar{Y}_{qr} \dist{\ntvar{Z}}_{rt},\forall r,t \in \states$;
\end{itemize}
The function $\phi \colon \dom{}(\yield) \rightarrow \dom{}(\yield')$ is defined as $\phi (q_\init,\ntvar{S}[q'_\init,\NTvar{S}],\str)=(\ntvar{S}_{q_\init q_\final}[q'_\init,\NTvar{S}],\str)$.
\end{proof}

\begin{proposition}\label{prop:ldpda-pda-eq-ldpda-cfg}
An LD-PDA controlled by a PDA is \bijeqJJ{} to an LD-PDA controlled by a CFG.
\end{proposition}

\begin{proof}
$(\Rightarrow)$ Let $\pushdown$ be an LD-PDA, $\pushdown'=(\states,\labelset,\stackalphabet,\trans,(q_\init,\NTvar{S}),(q_\final,\varepsilon))$ a controller PDA in normal form and $\yield$ the yield of $\pushdown$ controlled by $\pushdown'$. We define the controller CFG in normal form $\grammar=(\labelset,\stackalphabet',\rules,\NTvar{S})$, where $\stackalphabet'=\{\NTvar{X}_{pq}\mid \NTvar{X} \in \stackalphabet,p,q\in\states \}$ and the set of productions $\rules$ of $\grammar$ can be constructed as follows:
\begin{itemize}
    \item For each transition $p,\NTvar{X} \xrightarrow{\symvar{a}} q,\varepsilon$ add a production $\NTvar{X}_{pq} \rightarrow \symvar{a}$;
    \item For each transition $p,\ntvar{X} \xrightarrow{\varepsilon} q, \NTvar{Y}$ add productions $\ntvar{X}_{pr} \rightarrow \NTvar{Y}_{qr},\forall r \in \states$;
    \item For each transition $p,\NTvar{X} \xrightarrow{\varepsilon} q, \NTvar{Y} \ntvar{Z}$ add productions $\NTvar{X}_{pt} \rightarrow \NTvar{Y}_{qr} \NTvar{Z}_{rt},\forall r,t \in \states$;
    \item For each transition $p,\NTvar{X} \xrightarrow{\varepsilon} q, \NTvar{Y} \NTvar{Z}$ add productions $\NTvar{X}_{pt} \rightarrow \NTvar{Y}_{qr} \NTvar{Z}_{rt},\forall r,t \in \states$;
\end{itemize}
The yield of $\pushdown$ controlled by $\grammar$ is $\yield'$. The function $\phi \colon \dom{}(\yield) \rightarrow \dom{}(\yield')$ is defined as $\phi (q_\init,\ntvar{S}[q'_\init,\NTvar{S}],\str)=(q_\init,\ntvar{S}[\NTvar{S}_{q_\init q_\final}],\str)$.

$(\Leftarrow)$ Let $\pushdown$ be an LD-PDA, $\grammar=(\nonterm,\labelset,\rules,\NTvar{S})$ a controller CFG and $\yield$ the yield of $\pushdown$ controlled by $\grammar$. We define the controller PDA in normal form $\pushdown'=(\{p\},\labelset,\nonterm,\trans,(p,\NTvar{S}),(p,\varepsilon))$. For a controller CFG in normal form with productions 
\begin{align*}
    \NTvar{A} &\rightarrow \NTvar{BC},\\
    \NTvar{A} &\rightarrow \NTvar{B},\\
    \NTvar{A} &\rightarrow \ell,\\
    \NTvar{A} &\rightarrow \varepsilon,
\end{align*}
the set $\trans$ contains the transitions
\begin{align*}
    p,\NTvar{A} &\xrightarrow{\varepsilon}p, \NTvar{BC},\\
    p,\NTvar{A} &\xrightarrow{\varepsilon}p, \NTvar{B},\\
    p,\NTvar{A} &\xrightarrow{\ell}p, \varepsilon,\\
    p,\NTvar{A} &\xrightarrow{\varepsilon}p,\varepsilon.
\end{align*}
The yield of $\pushdown$ controlled by $\pushdown'$ is $\yield'$. The function $\phi \colon \dom{}(\yield) \rightarrow \dom{}(\yield')$ is defined as $\phi (q_\init,\ntvar{S}[\NTvar{S}],\str)=(q_\init,\ntvar{S}[p,\NTvar{S}],\str)$.
\end{proof}

\begin{proposition}\label{prop:ldpda-cfg-eq-ldcfg-cfg}
An LD-PDA controlled by a CFG is \bijeqJJ{} to an LD-CFG controlled by a CFG.
\end{proposition}

\begin{proof}
$(\Rightarrow)$ Let $\pushdown=(\states,\alphabet,\stackalphabet,\labelset,\trans,(q_\init,\ntvar{S}),(q_\final,\varepsilon))$ be an LD-PDA, $\grammar$ a controller CFG in normal form and $\yield$ the yield function of $\pushdown$ controlled by $\grammar$. We define the LD-CFG $\grammar'=(\nonterm,\alphabet,\labelset,\rules,\ntvar{S}_{q\init q_\final})$, where $\nonterm = \{\ntvar{X}_{pq} \mid \ntvar{X} \in \stackalphabet, p,q \in \states \}$. If $\pushdown$ is in normal form, the set of productions $\rules$ of $\grammar'$ can be constructed as follows:
\begin{itemize}
    \item For each transition $\ell \colon p,\ntvar{X} \xrightarrow{\symvar{a}} q,\varepsilon$ add a production $\ell \colon \ntvar{X}_{pq} \rightarrow \symvar{a}$;
    \item For each transition $\ell \colon p,\ntvar{X} \xrightarrow{\varepsilon} q, \dist{\ntvar{Y}}$ add productions $\ell \colon \ntvar{X}_{pr} \rightarrow \dist{\ntvar{Y}}_{qr},\forall r \in \states$;
    \item For each transition $\ell \colon p,\ntvar{X} \xrightarrow{\varepsilon} q, \dist{\ntvar{Y}} \ntvar{Z}$ add productions $\ell \colon \ntvar{X}_{pt} \rightarrow \dist{\ntvar{Y}}_{qr} \ntvar{Z}_{rt},\forall r,t \in \states$;
    \item For each transition $\ell \colon p,\ntvar{X} \xrightarrow{\varepsilon} q, \ntvar{Y} \dist{\ntvar{Z}}$ add productions $\ell \colon \ntvar{X}_{pt} \rightarrow \ntvar{Y}_{qr} \dist{\ntvar{Z}}_{rt},\forall r,t \in \states$;
\end{itemize}
The yield of $\grammar'$ controlled by $\grammar$ is $\yield'$. The function $\phi \colon \dom{}(\yield) \rightarrow \dom{}(\yield')$ is defined as $\phi (q_\init,\ntvar{S}[\NTvar{S}],\str)=(\ntvar{S}_{q_\init q_\final}[\NTvar{S}],\str)$.

$(\Leftarrow)$ Let $\grammar=(\nonterm,\alphabet,\labelset,\rules,\ntvar{S})$ be an LD-CFG in normal form, $\grammar'$ a controller CFG and $\yield$ the yield of $\grammar$ controlled by $\grammar'$. We define the LD-PDA $\pushdown=(\{p\},\alphabet,\nonterm,\labelset,\trans,(p,\ntvar{S}),(p,\varepsilon))$. For an LD-CFG in normal form with productions $\rules$
\begin{align*}
    \ell_1 \colon \ntvar{X} &\rightarrow \dist{\ntvar{Y}} \ntvar{Z},\\
    \ell_2 \colon \ntvar{X} &\rightarrow \ntvar{Y} \dist{\ntvar{Z}},\\
    \ell_3 \colon \ntvar{X} &\rightarrow \dist{\ntvar{Y}},\\
    \ell_4 \colon \ntvar{X} &\rightarrow \symvar{a},\\
    \ell_5 \colon \ntvar{X} &\rightarrow \varepsilon,
\end{align*}
we define the set of transitions $\trans$ as
\begin{align*}
    \ell_1 \colon p,\ntvar{X} &\xrightarrow{\varepsilon} p,\dist{\ntvar{Y}} \ntvar{Z},\\
    \ell_2 \colon p,\ntvar{X} &\xrightarrow{\varepsilon} p,\ntvar{Y} \dist{\ntvar{Z}},\\
    \ell_3 \colon p,\ntvar{X} &\xrightarrow{\varepsilon} p,\dist{\ntvar{Y}},\\
    \ell_4 \colon p,\ntvar{X} &\xrightarrow{\symvar{a}} p,\varepsilon,\\
    \ell_5 \colon p,\ntvar{X} &\xrightarrow{\varepsilon} p,\varepsilon.
\end{align*}
The yield of $\pushdown$ controlled by $\grammar'$ is $\yield'$. We define the function $\phi \colon \dom{}(\yield) \rightarrow \dom{}(\yield')$ as $\phi (\ntvar{S}[\NTvar{S}],\str)=(\ntvar{S}[p,\NTvar{S}],\str)$.
\end{proof}

\begin{proposition}
LD-CFGs controlled by CFGs, LD-CFGs controlled by PDAs, LD-PDAs controlled by CFGs and LD-PDAs controlled by PDAs are \bijeqJJ{}.
\end{proposition}

\begin{proof}
Proven by \cref{prop:ldcfg-cfg-eq-ldcfg-pda}, \cref{prop:ldcfg-pda-eq-ldpda-pda}, \cref{prop:ldpda-pda-eq-ldpda-cfg} and \cref{prop:ldpda-cfg-eq-ldcfg-cfg}.
\end{proof}

\section{\TopeqNN{}}\label{app:d-strong-eq}

We prove that LD-CFGs controlled by CFGs, LD-CFGs controlled by PDAs, LD-PDAs controlled by CFGs and LD-PDAs controlled by PDAs are \topeqJJ{} to TAG, LIG, PAA and EPDA, respectively.

\begin{proposition}
A tree-adjoining grammar is \topeqJJ{} to an LD-CFG controlled by a CFG.
\end{proposition}

\begin{proof}
    
\end{proof}

\begin{proposition}
A linear indexed grammar is \topeqJJ{} to an LD-CFG controlled by a PDA.
\end{proposition}

\begin{proof}
$(\Rightarrow)$ Let $\grammar=(\nonterm,\alphabet,\stackalphabet,\ntvar{S},\rules)$ be a LIG in normal form with the carrier set $\carrierset$ and yield function $\yield$. We can construct an LD-CFG $\grammar'=(\nonterm,\alphabet,\labelset,\rules',\ntvar{S})$ controlled by a PDA $\pushdown=(\{p\},\labelset,\trans,(p,\NTvar{S}),(p,\varepsilon))$ with the carrier set $\carrierset'$ and the yield function $\yield'$. 
\begin{itemize}
    \item For each rule $\ntvar{X}[\rest \NTvar{A}] \rightarrow \ntvar{X}[\rest \stackseq] \in \rules$, add the transition $p, \NTvar{A} \xrightarrow{\varepsilon} p, \stackseq$ to $\trans$.
    \item For each rule $\ntvar{X}[\rest \NTvar{A}] \rightarrow \ntvar{Y}[\rest] \in \rules$, add a new label $\ell$ to $\labelset$, the transition $p, \NTvar{A} \xrightarrow{\ell} p, \varepsilon$ to $\trans$ and the production $\ell \colon \ntvar{X} \rightarrow \dist{\ntvar{Y}}$ to $\rules'$.
    \item For each rule $\ntvar{X}[\rest \NTvar{A}] \rightarrow \ntvar{Y}[\rest] \ntvar{Z}[\NTvar{S}] \in \rules$, add a new label $\ell$ to $\labelset$, the transition $p, \NTvar{A} \xrightarrow{\ell} p, \varepsilon$ to $\trans$ and the production $\ell \colon \ntvar{X} \rightarrow \dist{\ntvar{Y}} \ntvar{Z}$ to $\rules'$.
    \item For each rule $\ntvar{X}[\rest \NTvar{A}] \rightarrow  \ntvar{Y}[\NTvar{S}] \ntvar{Z}[\rest] \in \rules$, add a new label $\ell$ to $\labelset$, the transition $p, \NTvar{A} \xrightarrow{\ell} p, \varepsilon$ to $\trans$ and the production $\ell \colon \ntvar{X} \rightarrow \ntvar{Y} \dist{\ntvar{Z}}$ to $\rules'$.
    \item For each rule $\ntvar{X}[\NTvar{A}] \rightarrow \symvar{a} \in \rules$, add a new label $\ell$ to $\labelset$, the transition $p, \NTvar{A} \xrightarrow{\ell} p, \varepsilon$ to $\trans$ and the production $\ell \colon \ntvar{X} \rightarrow \symvar{a}$ to $\rules'$.
\end{itemize}
We define the function $\phi \colon \carrierset \rightarrow \carrierset'$ as $\phi(\ntvar{X}[\stackseq],\str)=(\ntvar{X}[p,\stackseq],\str)$. $\carrierset$ and $\carrierset'$ have the same signature, $\phi$ is an isomorphism and $\yield = \yield' \circ \phi$.

$(\Leftarrow)$ Let $\grammar=(\nonterm,\alphabet,\labelset,\rules,\ntvar{S})$ be an LD-CFG controlled by a PDA $\pushdown=(\states,\labelset,\trans,(q_\init,\NTvar{S}),(q_\final,\varepsilon))$ with the carrier set $\carrierset$ and the yield function $\yield$. We construct the LIG $\grammar'=(\nonterm',\alphabet,\stackalphabet,\ntvar{S},\rules')$ where $\nonterm' = \{\ntvar{X}_p \mid \ntvar{X} \in \nonterm, p \in \states \}$ and the set of rules $\rules'$ such that
\begin{itemize}
    \item For each rule $p, \NTvar{A} \xrightarrow{\varepsilon} q, \stackseq \in \trans$, $\rules'$ contains a rule $\ntvar{X}_p[\rest \NTvar{A}] \rightarrow \ntvar{X}_q[\rest \stackseq], \forall \ntvar{X} \in \nonterm$.
    \item For each pair of rules $p, \NTvar{A} \xrightarrow{\ell} q, \varepsilon \in \trans$ and $\ell \colon \ntvar{X}\rightarrow \dist{\ntvar{Y}} \in \rules$, $\rules'$ contains a rule $\ntvar{X}_p[\rest \NTvar{A}] \rightarrow \ntvar{Y}_q[\rest]$.
    \item For each pair of rules $p, \NTvar{A} \xrightarrow{\ell} q, \varepsilon \in \trans$ and $\ell \colon \ntvar{X}\rightarrow \dist{\ntvar{Y}} \ntvar{Z} \in \rules$, $\rules'$ contains a rule $\ntvar{X}_p[\rest \NTvar{A}] \rightarrow \ntvar{Y}_q[\rest] \ntvar{Z}_{q_\init}[\NTvar{S}]$.
    \item For each pair of rules $p, \NTvar{A} \xrightarrow{\ell} q, \varepsilon \in \trans$ and $\ell \colon \ntvar{X}\rightarrow \ntvar{Y} \dist{\ntvar{Z}} \in \rules$, $\rules'$ contains a rule $\ntvar{X}_p[\rest \NTvar{A}] \rightarrow \ntvar{Y}_{q_\init}[\NTvar{S}] \ntvar{Z}_q[\rest]$.
    \item For each pair of rules $p, \NTvar{A} \xrightarrow{\ell} q_f, \varepsilon \in \trans$ and $\ell \colon \ntvar{X}\rightarrow \symvar{a} \in \rules$, $\rules'$ contains a rule $\ntvar{X}_p[\NTvar{A}] \rightarrow \symvar{a}$.
\end{itemize}
We define the function $\phi \colon \carrierset \rightarrow \carrierset'$ as $\phi(\ntvar{X}[p,\stackseq],\str)=(\ntvar{X}_p[\stackseq],\str)$. $\carrierset$ and $\carrierset'$ have the same signature, $\phi$ is an isomorphism and $\yield = \yield' \circ \phi$.
\end{proof}

\begin{proposition}
An embedded pushdown automaton is \topeqJJ{} to an LD-PDA controlled by a PDA.
\end{proposition}

\begin{proof}
$(\Rightarrow)$ Let $\pushdown=(\states,\alphabet,\nonterm,\stackalphabet,\trans,(q_0,\ntvar{S}[\NTvar{S}]),(q_f,\varepsilon))$ be an EPDA in normal form with carrier set $\carrierset$ and yield function $\yield$. We can construct an LD-PDA $\pushdown'=(\states,\alphabet,\labelset,\nonterm,\trans',(q_0,\ntvar{S}),(q_f,\varepsilon))$ controlled by a PDA $\pushdown''=(\{p\},\labelset,\stackalphabet,\trans'',(p,\NTvar{S}),(p,\varepsilon))$, with carrier set $\carrierset'$ and yield $\yield'$. The signature $\signature$ is constructed as follows:
\begin{itemize}
    \item For each transition $q, \nestedstack \ntvar{X}[\rest \NTvar{A}]\xrightarrow{\varepsilon} r, \nestedstack \ntvar{X}[\rest \stackseq] \in \trans, |\stackseq| \in \range{1}{2}$, add the transition $p, \NTvar{A} \xrightarrow{\varepsilon} p, \stackseq$ to $\trans'$.
    \item For each transition $q, \nestedstack \ntvar{X}[\rest \NTvar{A}]\xrightarrow{\varepsilon} r, \nestedstack \ntvar{Y} [\rest] \in \trans$, add a label $\ell$ to $\labelset$, the  transition $\ell \colon q, \ntvar{X} \xrightarrow{\varepsilon} r, \dist{\ntvar{Y}}$ to $\trans'$ and the transition $p, \NTvar{A} \xrightarrow{\ell} p, \varepsilon$ to $\trans'$.
    \item For each transition $q, \nestedstack \ntvar{X} [\rest \NTvar{A}]\xrightarrow{\varepsilon} r, \nestedstack \ntvar{Y} [\rest ]\ntvar{Z}[\NTvar{S}] \in \trans$, add a label $\ell$ to $\labelset$, the  transition $\ell \colon q, \ntvar{X} \xrightarrow{\varepsilon} r, \dist{\ntvar{Y}} \ntvar{Z}$ to $\trans'$ and the transition $p, \NTvar{A} \xrightarrow{\ell} p, \varepsilon$ to $\trans'$.
    \item For each transition $q, \nestedstack \ntvar{X}[\rest \NTvar{A}]\xrightarrow{\varepsilon} r, \nestedstack \ntvar{Y}[\NTvar{S}]\ntvar{Z}[\rest] \in \trans$, add a label $\ell$ to $\labelset$, the  transition $\ell \colon q, \ntvar{X} \xrightarrow{\varepsilon} r, \ntvar{Y} \dist{\ntvar{Z}}$ to $\trans'$ and the transition $p, \NTvar{A} \xrightarrow{\ell} p, \varepsilon$ to $\trans'$.
    \item For each transition $q, \nestedstack \ntvar{X}[ \NTvar{A}]\xrightarrow{\symvar{a}} r, \nestedstack \in \trans$, add a label $\ell$ to $\labelset$, the  transition $\ell \colon q, \ntvar{X} \xrightarrow{\symvar{a}} r, \varepsilon$ to $\trans'$ and the transition $p, \NTvar{A} \xrightarrow{\ell} p, \varepsilon$ to $\trans'$.
\end{itemize}
We define the function $\phi\colon \carrierset \rightarrow \carrierset'$ as $\phi(q,\nestedstack,\str)=(q,\nestedstack',\str)$, where, if $\nestedstack=\ntvar{X}_1[\stackseq_1]\ldots\ntvar{X}_k[\stackseq_k]$ then $\nestedstack'=\ntvar{X}_1[p,\stackseq_1]\ldots \ntvar{X}_k[p,\stackseq_k]$. $\carrierset$ and $\carrierset'$ have the same signature, $\phi$ is an isomorphism and $\yield = \yield' \circ \phi$.

$(\Leftarrow)$ Let $\pushdown=(\states,\alphabet,\labelset,\stackalphabet,\trans,(q_\init,\ntvar{S}),(q_\final,\varepsilon))$ be an LD-PDA controlled by a PDA $\pushdown'=(\states',\labelset,\stackalphabet',\trans',(q'_\init,\NTvar{S}),(q'_\final,\varepsilon))$ with carrier set $\carrierset$ and yield function $\yield$. Define the set $\nonterm= \{ \ntvar{X}_p \mid \ntvar{X} \in \stackalphabet, p \in \states' \}$ We can construct an EPDA $\pushdown''=(\states,\alphabet,\nonterm, \stackalphabet',\trans'',(q_\init,\ntvar{S}[\NTvar{S}]),(q_\final,\varepsilon))$ that is \topeqJJ{} to $\pushdown$ controlled by $\pushdown'$, with carrier set $\carrierset'$ and yield $\yield'$. The set $\trans''$ is defined as follows:
\begin{itemize}
    \item For each transition $r,\NTvar{A}\xrightarrow{\varepsilon}s,\NTvar{BC} \in \trans'$, $\trans''$ contains a transition $p, \nestedstack \ntvar{X}_r[\rest \NTvar{A}]\xrightarrow{\varepsilon}p,\nestedstack \ntvar{X}_s[\rest \NTvar{B} \NTvar{C}]$.
    \item For each transition $r,\NTvar{A}\xrightarrow{\varepsilon}s,\NTvar{B} \in \trans'$, $\trans''$ contains a transition $p, \nestedstack \ntvar{X}_r[\rest \NTvar{A}\xrightarrow{\varepsilon}p,\nestedstack \ntvar{X}_s[\rest \NTvar{B}]$.
    \item For each transition $r,\NTvar{A}\xrightarrow{\varepsilon}s,\varepsilon \in \trans'$, $\trans''$ contains a transition $p, \nestedstack \ntvar{X}_r[\rest \NTvar{A}]\xrightarrow{\varepsilon}p,\nestedstack \ntvar{X}_s[\rest]$.
    % \item For each pair of transitions $r,\NTvar{A}\xrightarrow{\ell}s,\NTvar{BC} \in \trans'$ and $\ell \colon p, \ntvar{X}\xrightarrow{\varepsilon}q,\dist{\ntvar{Y}} \in \trans$, $\trans''$ contains a transition $p, \nestedstack [\rest \NTvar{A}_{ru\ntvar{XW}}]\xrightarrow{\varepsilon}q,\nestedstack [\rest \NTvar{B}_{st\ntvar{YZ}} \NTvar{C}_{tu\ntvar{ZW}}]$.
    % \item For each pair of transitions $r,\NTvar{A}\xrightarrow{\ell}s,\NTvar{B} \in \trans'$ and $\ell \colon p, \ntvar{X}\xrightarrow{\varepsilon}q,\dist{\ntvar{Y}} \in \trans$, $\trans''$ contains a transition $p, \nestedstack [\rest \NTvar{A}_{rt\ntvar{XZ}}]\xrightarrow{\varepsilon}q,\nestedstack [\rest \NTvar{B}_{st\ntvar{YZ}}]$.
    \item For each pair of transitions $r,\NTvar{A}\xrightarrow{\ell}s,\varepsilon \in \trans'$ and $\ell \colon p, \ntvar{X}\xrightarrow{\varepsilon}q,\dist{\ntvar{Y}} \in \trans$, $\trans''$ contains a transition $p, \nestedstack \ntvar{X}_r[\rest \NTvar{A}]\xrightarrow{\varepsilon}q,\nestedstack \ntvar{Y}_s[\rest]$.
    % \item For each pair of transitions $r,\NTvar{A}\xrightarrow{\ell}s,\NTvar{BC} \in \trans'$ and $\ell \colon p, \ntvar{X}\xrightarrow{\varepsilon}q,\dist{\ntvar{Y}} \ntvar{Z} \in \trans$, $\trans''$ contains a transition $p, \nestedstack [\rest \NTvar{A}_{ru\ntvar{XU}}]\xrightarrow{\varepsilon}q,\nestedstack [\rest \NTvar{B}_{st\ntvar{YW}} \NTvar{C}_{tu\ntvar{WU}}][\NTvar{S}_{q'_0 q'_f \ntvar{Z}\varepsilon}]$.
    % \item For each pair of transitions $r,\NTvar{A}\xrightarrow{\ell}s,\NTvar{B} \in \trans'$ and $\ell \colon p, \ntvar{X}\xrightarrow{\varepsilon}q,\dist{\ntvar{Y}}\ntvar{Z} \in \trans$, $\trans''$ contains a transition $p, \nestedstack [\rest \NTvar{A}_{rt\ntvar{XW}}]\xrightarrow{\varepsilon}q,\nestedstack [\rest \NTvar{B}_{st\ntvar{YW}}][\NTvar{S}_{q'_0 q'_f \ntvar{Z}\varepsilon}]$.
    \item For each pair of transitions $r,\NTvar{A}\xrightarrow{\ell}s,\varepsilon \in \trans'$ and $\ell \colon p, \ntvar{X}\xrightarrow{\varepsilon}q,\dist{\ntvar{Y}} \ntvar{Z}\in \trans$, $\trans''$ contains a transition $p, \nestedstack \ntvar{X}_r[\rest \NTvar{A}]\xrightarrow{\varepsilon}q,\nestedstack \ntvar{Y}_s[\rest]\ntvar{Z}_{q'_\init}[\NTvar{S}]$.
    % \item For each pair of transitions $r,\NTvar{A}\xrightarrow{\ell}s,\NTvar{BC} \in \trans'$ and $\ell \colon p, \ntvar{X}\xrightarrow{\varepsilon}q,\ntvar{Y} \dist{\ntvar{Z}} \in \trans$, $\trans''$ contains a transition $p, \nestedstack [\rest \NTvar{A}_{ru\ntvar{XU}}]\xrightarrow{\varepsilon}q,\nestedstack [\NTvar{S}_{q'_0 q'_f \ntvar{Y}\varepsilon}] [\rest \NTvar{B}_{st\ntvar{ZW}} \NTvar{C}_{tu\ntvar{WU}}]$.
    % \item For each pair of transitions $r,\NTvar{A}\xrightarrow{\ell}s,\NTvar{B} \in \trans'$ and $\ell \colon p, \ntvar{X}\xrightarrow{\varepsilon}q,\ntvar{Y} \dist{\ntvar{Z}} \in \trans$, $\trans''$ contains a transition $p, \nestedstack [\rest \NTvar{A}_{rt\ntvar{XW}}]\xrightarrow{\varepsilon}q,\nestedstack [\NTvar{S}_{q'_0 q'_f \ntvar{Y}\varepsilon}] [\rest \NTvar{B}_{st\ntvar{ZW}}]$.
    \item For each pair of transitions $r,\NTvar{A}\xrightarrow{\ell}s,\varepsilon \in \trans'$ and $\ell \colon p, \ntvar{X}\xrightarrow{\varepsilon}q,\ntvar{Y} \dist{\ntvar{Z}} \in \trans$, $\trans''$ contains a transition $p, \nestedstack \ntvar{X}_r[\rest \NTvar{A}]\xrightarrow{\varepsilon}q,\nestedstack \ntvar{Y}_s[\NTvar{S}] \ntvar{Z}_{q'_\init}[\rest]$.
    \item For each pair of transitions $r,\NTvar{A}\xrightarrow{\ell}q'_\final,\varepsilon \in \trans'$ and $\ell \colon p, \ntvar{X}\xrightarrow{\symvar{a}}q,\varepsilon \in \trans$, $\trans''$ contains a transition $p, \nestedstack \ntvar{X}_r[\rest \NTvar{A}]\xrightarrow{\symvar{a}}q,\nestedstack$.
\end{itemize}
We define the function $\phi\colon \carrierset \rightarrow \carrierset'$ as $\phi(q,\nestedstack,\str)=(q,\nestedstack',\str)$, where, if $\nestedstack=\ntvar{X}_1[p_1,\stackseq_1]\ldots\ntvar{X}_k[p_k,\stackseq_k]$ then $\nestedstack'=\ntvar{X}_{1 p_1}[\stackseq_1]\ldots \ntvar{X}_{k p_k}[\stackseq_k]$. $\carrierset$ and $\carrierset'$ have the same signature, $\phi$ is an isomorphism and $\yield = \yield' \circ \phi$.

\end{proof}

\begin{proposition}
A pushdown adjoining automaton is \topeqJJ{} to an LD-PDA controlled by a CFG.
\end{proposition}

\begin{proof}
    
\end{proof}

\section{Examples}\label{app:examples}

% \begin{example} \label{ex:controlled_cfg}
% The following LD-CFG is the same as \citet{weir-1992-geometric}'s example 2.2:
% \begin{align*}
% \Sym{\ell_1} \colon \nt{S_1} &\rightarrow \sym{a} \nt{\dist{S}_1}
% &\Sym{\ell_4} \colon \nt{S_1} &\rightarrow \nt{\dist{S}_1} \sym{b} \\
% \Sym{\ell_2} \colon \nt{S_1} &\rightarrow \sym{b} \nt{\dist{S}_1} 
% &\Sym{\ell_5} \colon \nt{S_1} &\rightarrow \varepsilon \\
% \Sym{\ell_3} \colon \nt{S_1} &\rightarrow \nt{\dist{S}_1} \sym{a} 
% \end{align*}
% \end{example}

% \begin{example}
% The following is a derivation of the string $\sym{abbabb}$ using the LD-CFG from \cref{ex:controlled_cfg}.
% \begin{align*}
% \nt{S_1}[\varepsilon], \emptyset
% &\xRightarrow{\ell_1} \sym{a} \nt{S_1}[\Sym{\ell_1}], \emptyset \\
% &\xRightarrow{\ell_2} \sym{ab} \nt{S_1}[\Sym{\ell_1} \Sym{\ell_2}], \emptyset \\
% &\xRightarrow{\ell_2} \sym{abb} \nt{S_1}[\Sym{\ell_1} \Sym{\ell_2} \Sym{\ell_2}], \emptyset \\
% &\xRightarrow{\ell_4} \sym{abb} \nt{S_1}[\Sym{\ell_1} \Sym{\ell_2} \Sym{\ell_2} \Sym{\ell_4}] \sym{b}, \emptyset \\
% &\xRightarrow{\ell_4} \sym{abb} \nt{S_1}[\Sym{\ell_1} \Sym{\ell_2} \Sym{\ell_2} \Sym{\ell_4} \Sym{\ell_4}] \sym{bb}, \emptyset \\
% &\xRightarrow{\ell_3} \sym{abb} \nt{S_1}[\Sym{\ell_1} \Sym{\ell_2} \Sym{\ell_2} \Sym{\ell_4} \Sym{\ell_4} \Sym{\ell_3}] \sym{abb}, \emptyset \\
% &\xRightarrow{\ell_5} \sym{abbabb}, \{ \Sym{\ell_1} \Sym{\ell_2} \Sym{\ell_2} \Sym{\ell_4} \Sym{\ell_4} \Sym{\ell_3} \Sym{\ell_5} \}.
% \end{align*}
% \end{example}

\begin{example} \label{ex:ldcfg-2nf}
Weir's example 2.2 in normal form has the following production rules:
\begin{align*}
\Sym{\ell_1}: \nt{S_1} &\rightarrow \nt{A} \nt{\dist{S}_1}
&\Sym{\ell_5}: \nt{S_1} &\rightarrow \varepsilon \\
\Sym{\ell_2}: \nt{S_1} &\rightarrow \nt{B} \nt{\dist{S}_1}
&\Sym{\ell_6}: \nt{A} &\rightarrow \sym{a} \\
\Sym{\ell_3}: \nt{S_1} &\rightarrow \nt{\dist{S}_1} \nt{A} 
&\Sym{\ell_7}: \nt{B} &\rightarrow \sym{b} \\
\Sym{\ell_4}: \nt{S_1} &\rightarrow \nt{\dist{S}_1} \nt{B}
\end{align*}
\end{example}

\begin{example} \label{ex:ldpda}
The LD-CFG from \cref{ex:controlled_cfg} can be converted into an LD-PDA that has the following transitions:
\begin{align*}
\Sym{\ell_1} \colon q_0, \nt{S_1} &\xrightarrow{\epsilon} q_0, \nt{A} \nt{\dist{S}_1}, 
&\Sym{\ell_5} \colon q_0, \nt{S_1} &\xrightarrow{\epsilon} q_0, \epsilon, \\
\Sym{\ell_2} \colon q_0, \nt{S_1} &\xrightarrow{\epsilon} q_0, \nt{B} \nt{\dist{S}_1}, 
&\Sym{\ell_6} \colon q_0, \nt{A} &\xrightarrow{\symvar{a}} q_0, \epsilon, \\
\Sym{\ell_3} \colon q_0, \nt{S_1} &\xrightarrow{\epsilon} q_0, \nt{\dist{S}_1} \nt{A}, 
&\Sym{\ell_7} \colon q_0, \nt{B} &\xrightarrow{\symvar{b}} q_0, \epsilon,\\
\Sym{\ell_4} \colon q_0, \nt{S_1} &\xrightarrow{\epsilon} q_0, \nt{\dist{S}_1} \nt{B}.
\end{align*}
\end{example}

\begin{example} \label{ex:controller-cfg-2nf}
The CFG with the production rules
\begin{align*}
    \NT{S_2} &\rightarrow \NT{T} \Sym{\ell_5} 
    &\NT{T} &\rightarrow \varepsilon \\
    \NT{T} &\rightarrow \Sym{\ell_1} \NT{T} \Sym{\ell_3} 
    &\NT{T} &\rightarrow \Sym{\ell_2} \NT{T} \Sym{\ell_4}
\end{align*}
is the  same CFG from Weir's example 2.2. If we convert it to the normal form we get the following transitions:
\begin{align*}
    \NT{L_1} &\rightarrow \Sym{\ell_1} 
    &\NT{L_2} &\rightarrow \Sym{\ell_2} 
    &\NT{L_3} &\rightarrow \Sym{\ell_3} \\
    \NT{L_4} &\rightarrow \Sym{\ell_4} 
    &\NT{L_5} &\rightarrow \Sym{\ell_5} 
    &\NT{S_2} &\rightarrow \NT{T} \NT{L_5} \\
    \NT{T} &\rightarrow \varepsilon 
    &\NT{T} &\rightarrow \NT{L_6} \NT{L_3} 
    &\NT{L_6} &\rightarrow \NT{L_1} \NT{T} \\
    \NT{T} &\rightarrow \NT{L_7} \NT{L_4} 
    &\NT{L_7} &\rightarrow \NT{L_2} \NT{T}
\end{align*}
\end{example}

\begin{example}
The LD-CFG in normal form from \cref{ex:ldcfg-2nf} and the controller CFG from \cref{ex:controller-cfg-2nf} generate the tree rewriting rules from \cref{fig:weir-example-tree-rules}. \cref{fig:tag-derivation} shows a derivation of the string ``abab" using these rules.

\begin{figure}
\centering
\footnotesize
\begin{subfigure}[b]{0.15\textwidth}
\centering
$\NT{S_2} \rightarrow$
\Tree [.{$\NT{T}$} {$\NT{L_5}^*$} ]
\end{subfigure} 
\begin{subfigure}[b]{0.15\textwidth}
\centering
$\NT{T} \rightarrow$
\Tree [.{$\NT{L_6}$} {$\NT{L_3}^*$} ]
\end{subfigure} 
\begin{subfigure}[b]{0.15\textwidth}
\centering
$\NT{L_6} \rightarrow$
\Tree [.{$\NT{L_1}$} {$\NT{T}^*$} ]
\end{subfigure} 
\begin{subfigure}[b]{0.15\textwidth}
\centering
$\NT{T} \rightarrow$
\Tree [.{$\NT{L_7}$} {$\NT{L_4}^*$} ]
\end{subfigure} 
\begin{subfigure}[b]{0.15\textwidth}
\centering
$\NT{L_7} \rightarrow$
\Tree [.{$\NT{L_2}$} {$\NT{T}^*$} ]
\end{subfigure} 
\begin{subfigure}[b]{0.15\textwidth}
\centering
$\NT{L_1} \rightarrow$
\Tree [.{$\nt{S_1}$} {$\nt{A}$} {$\nt{S_1}^*$} ]
\end{subfigure}
\begin{subfigure}[b]{0.15\textwidth}
\centering
$\NT{L_2} \rightarrow$
\Tree [.{$\nt{S_1}$} {$\nt{B}$} {$\nt{S_1}^*$} ]
\end{subfigure}
\begin{subfigure}[b]{0.15\textwidth}
\centering
$\NT{L_3} \rightarrow$
\Tree [.{$\nt{S_1}$} {$\nt{S_1}^*$} {$\nt{A}$} ]
\end{subfigure}
\begin{subfigure}[b]{0.15\textwidth}
\centering
$\NT{L_4} \rightarrow$
\Tree [.{$\nt{S_1}$} {$\nt{S_1}^*$} {$\nt{B}$} ]
\end{subfigure}
\begin{subfigure}[b]{0.15\textwidth}
\centering
$\NT{L_5} \rightarrow$
\Tree [.{$\nt{S_1}$} {$\varepsilon$} ]
\end{subfigure}
\begin{subfigure}[b]{0.15\textwidth}
\centering
% $\NT{L_6} \rightarrow$
\Tree [.{$\nt{A}$} {$\sym{a}$} ]
\end{subfigure}
\begin{subfigure}[b]{0.15\textwidth}
\centering
% $\NT{L_7} \rightarrow$
\Tree [.{$\nt{B}$} {$\sym{b}$} ]
\end{subfigure}
\caption{Tree rewriting rules generated by merging the rules of the LD-CFG from \cref{ex:ldcfg-2nf} and the controller CFG from \cref{ex:controller-cfg-2nf}.}
\label{fig:weir-example-tree-rules}
\end{figure}

\begin{figure*}
    \centering
    \footnotesize
    \begin{subfigure}[b]{0.15\textwidth}
        $\NT{S_2} \quad \Rightarrow$
     \end{subfigure}
     \begin{subfigure}[b]{0.15\textwidth}
        \Tree [.{$\NT{T}$} {$\NT{L_5}$} ]
        $ \quad \Rightarrow$
     \end{subfigure}
     \begin{subfigure}[b]{0.15\textwidth}
        \Tree [.{$\NT{T}$} [.{$\nt{S_1}$} {$\varepsilon$} ] ]
        $ \quad \Rightarrow$
     \end{subfigure}
     \begin{subfigure}[b]{0.15\textwidth}
        \Tree [.{$\NT{L_6}$} [.{$\NT{L_3}$} [.{$\nt{S_1}$} {$\varepsilon$} ] ] ]
        $ \quad \Rightarrow$
     \end{subfigure}
     \begin{subfigure}[b]{0.15\textwidth}
        \Tree [.{$\NT{L_1}$} [.{$\NT{T}$} [.{$\NT{L_3}$} [.{$\nt{S_1}$} {$\varepsilon$} ] ] ] ]
        $ \quad \Rightarrow$
     \end{subfigure}
     \begin{subfigure}[b]{0.15\textwidth}
        \Tree [.{$\NT{L_1}$} [.{$\NT{T}$} [.{$\nt{S_1}$} [.{$\nt{S_1}$} {$\varepsilon$} ] {$\nt{A}$} ] ] ]
        $ \quad \Rightarrow$
     \end{subfigure}
     \begin{subfigure}[b]{0.15\textwidth}
        \Tree [.{$\NT{L_1}$} [.{$\NT{T}$} [.{$\nt{S_1}$} [.{$\nt{S_1}$} {$\varepsilon$} ] [.{$a$} ] ] ] ]
        $ \quad \Rightarrow$
     \end{subfigure}
     \begin{subfigure}[b]{0.2\textwidth}
        \Tree [.{$\nt{S_1}$} {$\nt{A}$} [.{$\nt{S_1}$} [.{$\NT{T}$} [.{$\nt{S_1}$} [.{$\nt{S_1}$} {$\varepsilon$} ] [.{$a$} ] ] ] ] ]
        $ \quad \Rightarrow$
     \end{subfigure}
     \begin{subfigure}[b]{0.2\textwidth}
        \Tree [.{$\nt{S_1}$} [.{$a$} ] [.{$\nt{S_1}$} [.{$\NT{T}$} [.{$\nt{S_1}$} [.{$\nt{S_1}$} {$\varepsilon$} ] [.{$a$} ] ] ] ] ]
        $ \quad \Rightarrow$
     \end{subfigure}
     \begin{subfigure}[b]{0.2\textwidth}
        \Tree [.{$\nt{S_1}$} [.{$a$} ] [.{$\nt{S_1}$} [.{$\NT{L_7}$} [.{$\NT{L_4}$} [.{$\nt{S_1}$} [.{$\nt{S_1}$} {$\varepsilon$} ] [.{$a$} ] ] ] ] ] ]
        $ \quad \Rightarrow$
     \end{subfigure}
     \begin{subfigure}[b]{0.2\textwidth}
        \Tree [.{$\nt{S_1}$} [.{$a$} ] [.{$\nt{S_1}$} [.{$\NT{L_2}$} [.{$\NT{T}$} [.{$\NT{L_4}$} [.{$\nt{S_1}$} [.{$\nt{S_1}$} {$\varepsilon$} ] [.{$a$} ] ] ] ] ] ] ]
        $ \quad \Rightarrow$
     \end{subfigure}
         \begin{subfigure}[b]{0.2\textwidth}
        \Tree [.{$\nt{S_1}$} [.{$a$} ] [.{$\nt{S_1}$} [.{$\nt{S_1}$} [.{$\nt{S_1}$} {$\nt{B}$} [.{$\NT{T}$} [.{$\NT{L_4}$} [.{$\nt{S_1}$} [.{$\nt{S_1}$} {$\varepsilon$} ] [.{$a$} ] ] ] ] ] ] ] ]
        $ \quad \Rightarrow$
     \end{subfigure}
     \begin{subfigure}[b]{0.2\textwidth}
        \Tree [.{$\nt{S_1}$} [.{$a$} ] [.{$\nt{S_1}$} [.{$\nt{S_1}$} [.{$\nt{S_1}$} [.{$b$} ] [.{$\NT{T}$} [.{$\NT{L_4}$} [.{$\nt{S_1}$} [.{$\nt{S_1}$} {$\varepsilon$} ] [.{$a$} ] ] ] ] ] ] ] ]
        $ \quad \Rightarrow$
     \end{subfigure}
     \begin{subfigure}[b]{0.2\textwidth}
        \Tree [.{$\nt{S_1}$} [.{$a$} ] [.{$\nt{S_1}$} [.{$\nt{S_1}$} [.{$\nt{S_1}$} [.{$b$} ] [.{$\NT{T}$} [.{$\nt{S_1}$} [.{$\nt{S_1}$} [.{$\nt{S_1}$} [.{$\NT{S_1}$} {$\varepsilon$} ] [.{$a$} ] ] ] ] {$\nt{B}$} ] ] ] ] ]
        $ \quad \Rightarrow$
     \end{subfigure}
     \begin{subfigure}[b]{0.2\textwidth}
        \Tree [.{$\nt{S_1}$} [.{$a$} ] [.{$\nt{S_1}$} [.{$\nt{S_1}$} [.{$\nt{S_1}$} [.{$b$} ] [.{$\NT{T}$} [.{$\nt{S_1}$} [.{$\nt{S_1}$} [.{$\nt{S_1}$} [.{$\nt{S_1}$} {$\varepsilon$} ] [.{$a$} ] ] ] ] [.{$b$} ] ] ] ] ] ]
     \end{subfigure}
    \caption{Example of derivation in a CFG $\control$ CFG.}
    \label{fig:tag-derivation}
\end{figure*}
\end{example}

\begin{example} \label{ex:controller-pda-2nf} 
The controller CFG from \cref{ex:controller-cfg-2nf} can be converted into a controller PDA that recognizes the same language and has the transitions
\begin{align*}
p, \NT{T} &\xrightarrow{\varepsilon} p, \NT{L_1} \NT{T} \NT{L_3},
&p, \NT{S_2} &\xrightarrow{\varepsilon} p, \NT{T} \NT{L_5}, \\
p, \NT{T} &\xrightarrow{\varepsilon} p, \NT{L_2} \NT{T} \NT{L_4},
&p, \NT{T} &\xrightarrow{\varepsilon} p, \varepsilon,\\
p, \NT{L_i} &\xrightarrow{\Sym{\ell_i}} p, \varepsilon \quad (i\in\range{1}{5}). 
\end{align*}
By converting it to the normal form we get the following transitions:
\begin{align*}
p, \NT{S_2} &\xrightarrow{\varepsilon} p, \NT{T} \NT{L_5} 
&p, \NT{T} &\xrightarrow{\varepsilon} p, \varepsilon \\
p, \NT{T} &\xrightarrow{\varepsilon} p, \NT{L_6} \NT{L_3} 
&p, \NT{L_6} &\xrightarrow{\varepsilon} p, \NT{L_1} \NT{T} \\
p, \NT{T} &\xrightarrow{\varepsilon} p, \NT{L_7} \NT{L_4} 
&p, \NT{L_7} &\xrightarrow{\varepsilon} p, \NT{L_2} \NT{T} \\
p, \NT{L_i} &\xrightarrow{\Sym{\ell_i}} p, \varepsilon \quad (i\in\range{1}{5}).
\end{align*}
\end{example}

\begin{example}
    Consider the controller CFG with productions 
    \begin{align*}
        \NT{A} &\rightarrow \NT{B} \NT{C}\\
        \NT{B} &\rightarrow \NT{D} \NT{E} \\
        \NT{D} &\rightarrow \ell_1 \\
        \NT{E} &\rightarrow \ell_2 \\
        \NT{C} &\rightarrow \ell_3 \\
        \NT{A} &\rightarrow \ell_4 
    \end{align*}
    and the LD-CFG with productions 
    \begin{align*}
        &\ell_1 \colon \ntvar{X} \rightarrow \dist{\nt{Y}} \nt{Z} \\
        &\ell_2 \colon \ntvar{Y} \rightarrow \dist{\nt{W}} \\
        &\ell_3 \colon \ntvar{W} \rightarrow \sym{a} \\
        &\ell_4 \colon \ntvar{Z} \rightarrow \sym{b}
    \end{align*}
    By mixing the production rules in the two grammars we obtain the tree adjoining rules shown in \cref{fig:cfg-cfg-tree-rules}.
    \begin{figure}
        % \centering
        \begin{subfigure}[b]{0.2\textwidth}
        $\NT{D}_{\nt{X} \nt{Y}} \rightarrow$
        \Tree [.{$\nt{X}$} {$\nt{Y^*}$} {$\NT{S}_{\nt{Z}-}$} ]
     \end{subfigure}
    \begin{subfigure}[b]{0.2\textwidth}
        $\NT{E}_{\nt{Y} \nt{W}} \rightarrow$
        \Tree [.{$\nt{Y}$} {$\nt{W^*}$} ]
     \end{subfigure}
     \begin{subfigure}[b]{0.2\textwidth}
        $\NT{C}_{\nt{W} -} \rightarrow$
        \Tree [.{$\nt{W}$} {$\sym{a}$} ]
     \end{subfigure}
     \begin{subfigure}[b]{0.2\textwidth}
        $\NT{S}_{\nt{Z} -} \rightarrow$
        \Tree [.{$\nt{Z}$} {$\sym{b}$} ]
     \end{subfigure}
     \begin{subfigure}[b]{0.2\textwidth}
        $\NT{A}_{\nt{X} \nt{X}} \rightarrow$
        \Tree [.{$\NT{B}_{\nt{X} \nt{X}}$} {$\NT{C}_{\nt{W} -}$} ]
     \end{subfigure}
     \begin{subfigure}[b]{0.2\textwidth}
        $\NT{B}_{\nt{X} \nt{X}} \rightarrow$
        \Tree [.{$\NT{D}_{\nt{X} \nt{Y}}$} {$\NT{E}_{\nt{Y} \nt{W}}$} ]
     \end{subfigure}
        \caption{Tree adjoining rules obtained from a CFG controlling a CFG.}
        \label{fig:cfg-cfg-tree-rules}
    \end{figure}

    \begin{figure*}[!h]
        \begin{subfigure}[b]{0.15\textwidth}
        \centering
        \Tree [.{$\NT{A}_{\nt{X} \nt{X}}$} ]
        $\quad \Rightarrow$
     \end{subfigure}
     \begin{subfigure}[b]{0.15\textwidth}
     \centering
        \Tree [.{$\NT{B}_{\nt{X} \nt{X}}$} {$\NT{C}_{\nt{W} -}$} ]
        $\quad \Rightarrow$
     \end{subfigure}
     \begin{subfigure}[b]{0.15\textwidth}
     \centering
        \Tree [.{$\NT{D}_{\nt{X} \nt{Y}}$} [.{$\NT{E}_{\nt{Y} \nt{W}}$} {$\NT{C}_{\nt{W} -}$} ] ]
        $\quad \Rightarrow$
     \end{subfigure}
     \begin{subfigure}[b]{0.15\textwidth}
     \centering
        \Tree [.{$\nt{X}$} [.{$\NT{Y}$} [.{$\NT{E}_{\nt{Y} \nt{W}}$} {$\NT{C}_{\nt{W} -}$} ] ] {$\NT{S}_{\nt{Z}-}$} ]
        $\quad \Rightarrow$
     \end{subfigure}
     \begin{subfigure}[b]{0.15\textwidth}
     \centering
        \Tree [.{$\nt{X}$} [.{$\NT{Y}$} [.{$\nt{Y}$} [.{$\nt{W}$} {$\NT{C}_{\nt{W} -}$} ] ] ] [.{$\nt{Z}$} {$\sym{b}$} ] ]
        $\quad \Rightarrow$
     \end{subfigure}
     \begin{subfigure}[b]{0.15\textwidth}
     \centering
        \Tree [.{$\nt{X}$} [.{$\NT{Y}$} [.{$\nt{Y}$} [.{$\nt{W}$} [.{$\nt{W}$} {$\sym{a}$} ] ] ] ] [.{$\nt{Z}$} {$\sym{b}$} ] ]
     \end{subfigure}
     \caption{Derivation in the TAG with rules from \cref{fig:cfg-cfg-tree-rules}.}
    \label{fig:cfg-cfg-derivation}
    \end{figure*}
\end{example}
